# Supplementary material for: Large language models can be zero-shot anomaly detectors for time series?
Source: arXiv:2405.14755 source file (2024-10-31)
Supplement: Supplementary file 1 [file appendix.tex]

% \section{\prompt}

% \begin{figure}[ht]
%     \centering
%     \inputminted{python}{listings/gpt-code-example.py}
%     \vspace{3em}
%     \caption{Example code output from \gpt{} when prompted to find anomalies.}
%     \label{fig:gpt-code-example}
% \end{figure}

% \begin{minted}{python}
% import numpy as np

% def detect_anomalies(data, window_size, threshold):
%     moving_avg = np.convolve(data, np.ones(window_size)/window_size, mode='valid')
%     residual = data[window_size-1:] - moving_avg

%     std_dev = np.std(residual)
%     anomaly_indices = np.where(np.abs(residual) > threshold * std_dev)[0] + window_size - 1

%     return anomaly_indices

% # Example usage
% data = [...]
% window_size = 10
% threshold = 3
% anomaly_indices = detect_anomalies(data, window_size, threshold)
% print("Anomaly indices:", anomaly_indices)
% \end{minted}

% \section{Evaluation}

\begin{table*}[ht]
    \centering
    \caption{Performance of \mistral{} and \gpt{} models with \detect on a 5\% sample of the dataset.}
    \label{tab:detector_gpt}
    \begin{tabular}{l*{10}{c}r}
    \toprule
     & \multicolumn{5}{c}{\mistral{}} & \multicolumn{5}{c}{\gpt{}}\\
    \cmidrule(lr){2-6}\cmidrule(lr){7-11}
    \textbf{Dataset} & FP & FN & TP & time & F1 Score & FP & FN & TP & time & F1 Score & $\Delta$ F1 \\
    \midrule
    MSL     & 1 & 1 & 1 & 7.229 & 0.500 & 1 & 1 & 1 & 1.669 & 0.500 & 0.000 \\
    SMAP    & 2 & 3 & 1 & 22.18 & 0.285 & 1 & 3 & 1 & 4.299 & 0.333 & +0.048 \\
    A1      & 2 & 0 & 3 & 2.510 & 0.750 & 2 & 0 & 3 & 0.707 & 0.750 & 0.000\\
    A2      & 0 & 2 & 2 & 1.546 & 0.667 & 0 & 2 & 2 & 0.662 & 0.667 & 0.000\\
    A3      & 0 & 22 & 0 & 2.308 & 0.000 & 0 & 22 & 0 & 0.931 & 0.000 & 0.000\\
    A4      & 0 & 20 & 0 & 2.156 & 0.000 & 0 & 20 & 0 & 0.887 & 0.000 & 0.000 \\
    Art     & 0 & 2 & 0 & 5.591 & 0.000 & 0 & 2 & 0 & 1.965 & 0.000 & 0.000\\
    AWS     & 13 & 2 & 2 & 6.184 & 0.210 & 12 & 3 & 1 & 1.975 & 0.117 & -0.093\\
    AdEx    & 0 & 3 & 0 & 2.788 & 0.000 & 2 & 3 & 0 & 0.852 & 0.000 & 0.000 \\
    Traf    & 1 & 1 & 2 & 4.078 & 0.667 & 2 & 2 & 1 & 1.327 & 0.333 & -0.333\\
    Tweets  & 1 & 4 & 4 & 21.87 & 0.615 & 2 & 2 & 6 & 6.817 & 0.750 & +0.135\\
    \midrule
    Total   & 20 & 60 & 15 & 78.44 & 0.273 & 22 & 60 & 15 & 22.091 & 0.273 & 0.000 \\
    \bottomrule
    \end{tabular}
\end{table*}
\begin{table*}[!t]
\caption{Benchmark Summary Results}
\label{tab:all_experiments}
\resizebox{\linewidth}{!}{%
\begin{tabular}{lcccccccccccc}
\toprule
& \multicolumn{2}{c}{NASA} & \multicolumn{4}{c}{Yahoo S5} & \multicolumn{5}{c}{NAB}  \\
\cmidrule(r){2-3}\cmidrule(r){4-7}\cmidrule(r){8-12}
\textbf{Pipeline} & MSL & SMAP & A1 & A2 & A3 & A4 & Art & AWS & AdEx & Traf & Tweets & $\mu \pm \sigma$\\
\midrule
\multicolumn{12}{c}{\textbf{F1 Score}}\\
\midrule
\texttt{AER}        & 0.587 & 0.819 & 0.799 & 0.987 & 0.892 & 0.709 & 0.714 & 0.741 & 0.690 & 0.703 & 0.638 & 0.753 $\pm$ 0.109 \\
\texttt{LSTM DT}    & 0.471 & 0.726 & 0.728 & 0.985 & 0.744 & 0.646 & 0.400 & 0.468 & 0.786 & 0.585 & 0.603 & 0.649 $\pm$ 0.161 \\
\texttt{ARIMA}      & 0.525 & 0.411 & 0.728 & 0.856 & 0.797 & 0.686 & 0.308 & 0.382 & 0.727 & 0.467 & 0.514 & 0.582 $\pm$ 0.176 \\
\texttt{ARIMA}      & 0.474 & 0.423 & 0.507 & 0.897 & 0.793 & 0.825 & 0.571 & 0.440 & 0.692 & 0.305 & 0.343 & 0.570 $\pm$ 0.193 \\
\texttt{TadGAN}     & 0.560 & 0.605 & 0.578 & 0.817 & 0.416 & 0.340 & 0.500 & 0.623 & 0.818 & 0.452 & 0.554 & 0.569 $\pm$ 0.142 \\
\texttt{LSTM AE}    & 0.545 & 0.662 & 0.595 & 0.867 & 0.466 & 0.239 & 0.667 & 0.741 & 0.500 & 0.500 & 0.475 & 0.569 $\pm$ 0.158 \\
\texttt{VAE}        & 0.494 & 0.613 & 0.592 & 0.803 & 0.438 & 0.230 & 0.667 & 0.689 & 0.583 & 0.483 & 0.533 & 0.557 $\pm$ 0.143 \\
\texttt{LNN}        & 0.517 & 0.618 & 0.652 & 0.938 & 0.331 & 0.191 & 0.375 & 0.481 & 0.714 & 0.667 & 0.575 & 0.551 $\pm$ 0.196 \\
\texttt{Dense AE}   & 0.559 & 0.692 & 0.667 & 0.892 & 0.070 & 0.101 & 0.545 & 0.764 & 0.600 & 0.563 & 0.508 & 0.542 $\pm$ 0.240 \\
\texttt{AT}         & 0.400 & 0.266 & 0.571 & 0.565 & 0.760 & 0.576 & 0.414 & 0.430 & 0.500 & 0.371 & 0.287 & 0.467 $\pm$ 0.138 \\
\texttt{MV}         & 0.171 & 0.092 & 0.713 & 0.356 & 0.647 & 0.615 & 0.222 & 0.408 & 0.880 & 0.157 & 0.776 & 0.458 $\pm$ 0.266 \\
\texttt{GANF}       & 0.462 & 0.463 & 0.086 & 0.171 & 0.008 & 0.152 & 0.667 & 0.578 & 0.308 & 0.583 & 0.667 & 0.377 $\pm$ 0.230 \\
\texttt{MS Azure}   & 0.051 & 0.019 & 0.280 & 0.653 & 0.702 & 0.344 & 0.056 & 0.112 & 0.163 & 0.117 & 0.176 & 0.243 $\pm$ 0.225 \\
\midrule
\prompt \mistral{}  & 0.160 & 0.154 & 0.194 & 0.235 & 0.338 & 0.336 & 0.370 & 0.268 & 0.000 & 0.135 & 0.257 & 0.223 $\pm$ 0.104 \\
\prompt \gpt{}      & 0.049 & 0.110 & 0.143 & 0.078 & 0.157 & 0.195 & 0.154 & 0.194 & 0.133 & 0.133 & 0.000 & 0.122 $\pm$ 0.057 \\
\detect             & 0.429 & 0.431 & 0.615 & 0.828 & 0.376 & 0.363 & 0.400 & 0.362 & 0.727 & 0.480 & 0.762 & 0.525 $\pm$ 0.167 \\
\midrule
\multicolumn{12}{c}{\textbf{Precision}}\\
\midrule
\texttt{AER}        & 0.564 & 0.867 & 0.830 & 0.990 & 0.993 & 0.917 & 0.625 & 0.833 & 0.556 & 0.565 & 0.611 & 0.759 $\pm$ 0.168 \\
\texttt{LSTM DT}    & 0.364 & 0.671 & 0.665 & 0.985 & 0.986 & 0.905 & 0.333 & 0.383 & 0.647 & 0.444 & 0.550 & 0.630 $\pm$ 0.232 \\
\texttt{ARIMA}      & 0.477 & 0.303 & 0.670 & 0.769 & 0.998 & 0.955 & 0.286 & 0.342 & 0.727 & 0.438 & 0.486 & 0.586 $\pm$ 0.241 \\
\texttt{MP}         & 0.346 & 0.291 & 0.448 & 0.824 & 0.952 & 0.946 & 0.500 & 0.314 & 0.600 & 0.200 & 0.324 & 0.522 $\pm$ 0.259 \\
\texttt{TadGAN}     & 0.538 & 0.516 & 0.629 & 0.845 & 0.762 & 0.588 & 0.400 & 0.613 & 0.818 & 0.412 & 0.562 & 0.608 $\pm$ 0.142 \\
\texttt{LSTM AE}    & 0.512 & 0.615 & 0.633 & 0.827 & 0.948 & 0.649 & 0.667 & 0.833 & 0.462 & 0.444 & 0.538 & 0.648 $\pm$ 0.155 \\
\texttt{VAE}        & 0.444 & 0.600 & 0.574 & 0.701 & 0.852 & 0.646 & 0.667 & 0.677 & 0.538 & 0.467 & 0.593 & 0.615 $\pm$ 0.109 \\
\texttt{LNN}        & 0.434 & 0.520 & 0.632 & 0.895 & 0.954 & 0.590 & 0.300 & 0.388 & 0.588 & 0.500 & 0.525 & 0.575 $\pm$ 0.189 \\
\texttt{Dense AE}   & 0.594 & 0.714 & 0.748 & 0.939 & 0.944 & 0.590 & 0.600 & 0.840 & 0.667 & 0.500 & 0.577 & 0.701 $\pm$ 0.144 \\
\texttt{AT}         & 0.254 & 0.159 & 0.504 & 0.441 & 0.834 & 0.747 & 0.261 & 0.299 & 0.360 & 0.232 & 0.169 & 0.387 $\pm$ 0.216 \\
\texttt{MV}         & 0.093 & 0.048 & 0.573 & 0.217 & 0.589 & 0.534 & 0.125 & 0.259 & 0.786 & 0.085 & 0.635 & 0.359 $\pm$ 0.255 \\
\texttt{GANF}       & 0.750 & 0.786 & 0.281 & 0.300 & 1.000 & 0.986 & 1.000 & 0.867 & 1.000 & 0.700 & 0.639 & 0.755 $\pm$ 0.251 \\
\texttt{MS Azure}   & 0.026 & 0.009 & 0.167 & 0.484 & 0.542 & 0.217 & 0.029 & 0.060 & 0.089 & 0.062 & 0.099 & 0.162 $\pm$ 0.176 \\
\midrule
\prompt \mistral{}  & 0.286 & 0.292 & 0.178 & 0.200 & 0.389 & 0.358 & 0.238 & 0.194 & 0.000 & 0.080 & 0.191 & 0.219 $\pm$ 0.108 \\
\prompt \gpt{}      & 0.200 & 0.143 & 0.183 & 0.136 & 0.641 & 0.640 & 0.143 & 0.143 & 0.250 & 0.097 & 0.000 & 0.234 $\pm$ 0.201 \\
\detect             & 0.441 & 0.510 & 0.557 & 0.877 & 0.917 & 0.720 & 0.500 & 0.266 & 0.727 & 0.545 & 0.686 & 0.613 $\pm$ 0.184 \\
\midrule
\multicolumn{12}{c}{\textbf{Recall}}\\
\midrule
\texttt{AER}        & 0.611 & 0.776 & 0.770 & 0.985 & 0.809 & 0.578 & 0.833 & 0.667 & 0.909 & 0.929 & 0.667 & 0.776 $\pm$ 0.128 \\
\texttt{LSTM DT}    & 0.667 & 0.791 & 0.803 & 0.985 & 0.597 & 0.502 & 0.500 & 0.600 & 1.000 & 0.857 & 0.667 & 0.724 $\pm$ 0.168 \\
\texttt{ARIMA}      & 0.583 & 0.642 & 0.798 & 0.965 & 0.663 & 0.535 & 0.333 & 0.433 & 0.727 & 0.500 & 0.545 & 0.611 $\pm$ 0.168 \\
\texttt{MP}         & 0.750 & 0.776 & 0.584 & 0.985 & 0.679 & 0.732 & 0.667 & 0.733 & 0.818 & 0.643 & 0.364 & 0.703 $\pm$ 0.147 \\
\texttt{TadGAN}     & 0.583 & 0.731 & 0.534 & 0.790 & 0.286 & 0.240 & 0.667 & 0.633 & 0.818 & 0.500 & 0.545 & 0.575 $\pm$ 0.177 \\
\texttt{LSTM AE}    & 0.583 & 0.716 & 0.562 & 0.910 & 0.309 & 0.146 & 0.667 & 0.667 & 0.545 & 0.571 & 0.424 & 0.555 $\pm$ 0.196 \\
\texttt{VAE}        & 0.556 & 0.627 & 0.612 & 0.940 & 0.295 & 0.140 & 0.667 & 0.700 & 0.636 & 0.500 & 0.485 & 0.560 $\pm$ 0.201 \\
\texttt{LNN}        & 0.639 & 0.761 & 0.674 & 0.985 & 0.200 & 0.114 & 0.500 & 0.633 & 0.909 & 1.000 & 0.636 & 0.641 $\pm$ 0.274 \\
\texttt{Dense AE}   & 0.528 & 0.672 & 0.601 & 0.850 & 0.036 & 0.055 & 0.500 & 0.700 & 0.545 & 0.643 & 0.455 & 0.508 $\pm$ 0.241 \\
\texttt{AT}         & 0.944 & 0.821 & 0.657 & 0.785 & 0.698 & 0.469 & 1.000 & 0.767 & 0.818 & 0.929 & 0.939 & 0.802 $\pm$ 0.147 \\
\texttt{MV}         & 1.000 & 1.000 & 0.944 & 0.985 & 0.717 & 0.725 & 1.000 & 0.967 & 1.000 & 1.000 & 1.000 & 0.940 $\pm$ 0.105 \\
\texttt{GANF}       & 0.333 & 0.328 & 0.051 & 0.120 & 0.004 & 0.083 & 0.500 & 0.433 & 0.182 & 0.500 & 0.697 & 0.294 $\pm$ 0.213 \\
\texttt{MS Azure}   & 0.806 & 0.940 & 0.848 & 1.000 & 0.998 & 0.837 & 1.000 & 0.833 & 0.909 & 1.000 & 0.818 & 0.908 $\pm$ 0.078 \\
\midrule
\prompt \mistral{}  & 0.111 & 0.104 & 0.213 & 0.285 & 0.298 & 0.317 & 0.833 & 0.433 & 0.000 & 0.429 & 0.394 & 0.311 $\pm$ 0.213 \\
\prompt \gpt{}      & 0.028 & 0.090 & 0.118 & 0.055 & 0.089 & 0.115 & 0.167 & 0.300 & 0.091 & 0.214 & 0.197 & 0.133 $\pm$ 0.076 \\
\detect             & 0.417 & 0.373 & 0.685 & 0.785 & 0.236 & 0.243 & 0.333 & 0.567 & 0.727 & 0.429 & 0.857 & 0.514 $\pm$ 0.211 \\
\bottomrule
\end{tabular}}
\end{table*}

\begin{figure*}[ht]
    \centering
    \includegraphics[width=0.9\textwidth]{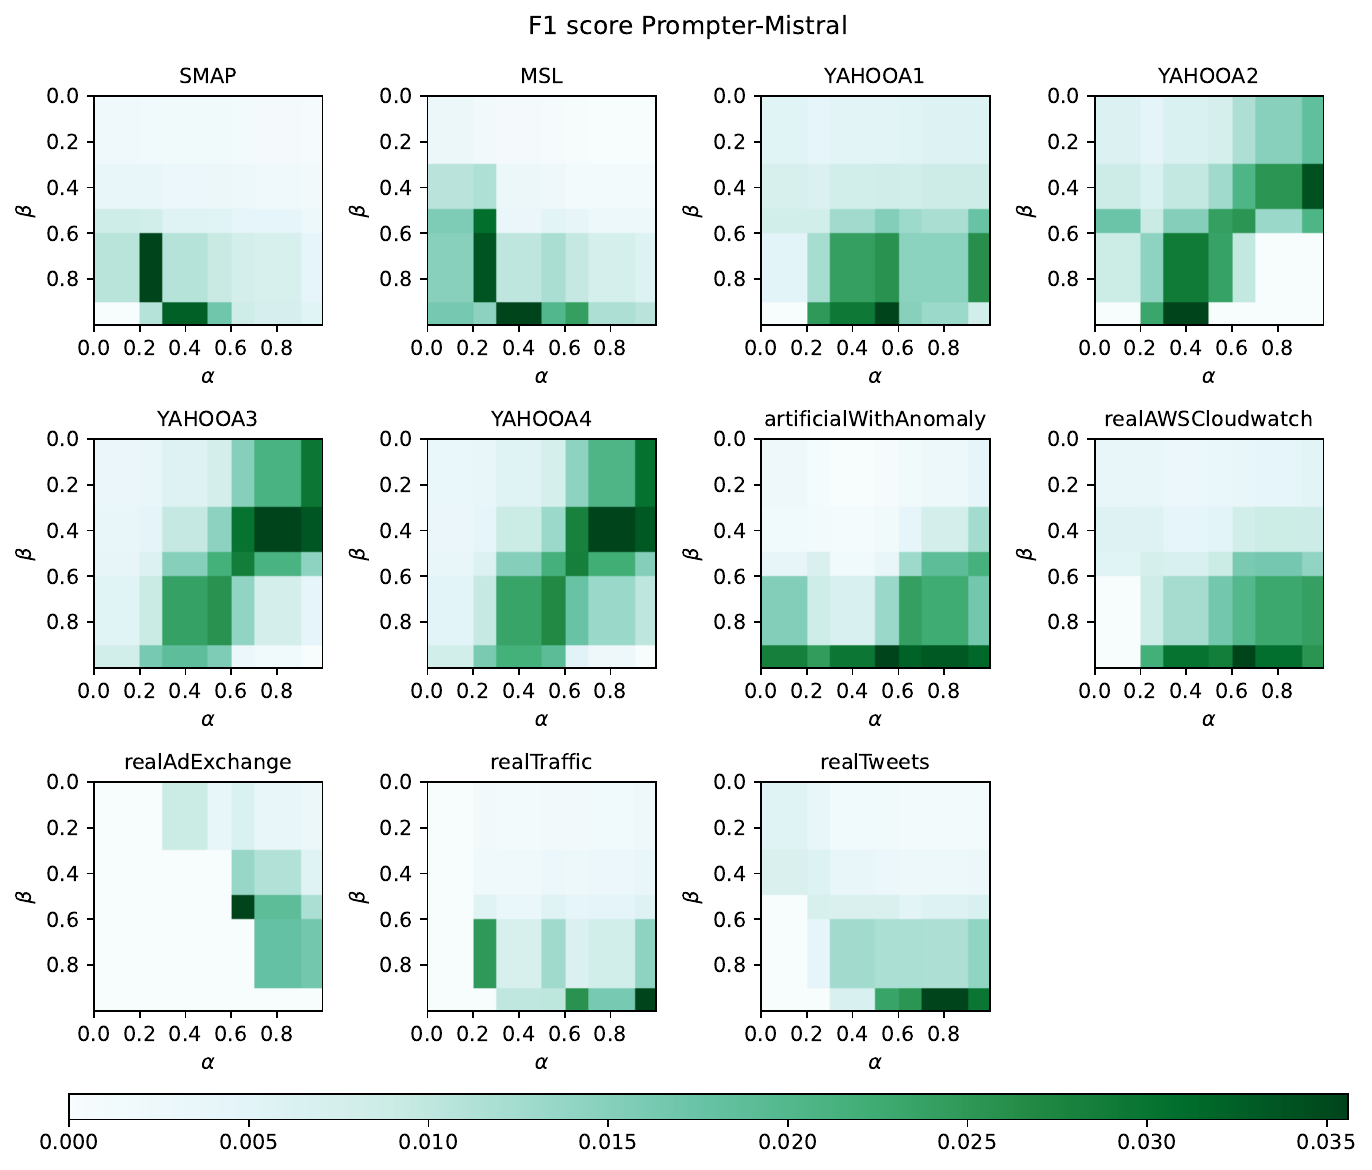}
    \caption{\prompt \mistral{} F1 score versus $\alpha$ and $\beta$ for each dataset.}
    \label{fig:mistral_prompter_dataset}
\end{figure*}

\begin{figure*}[ht]
    \centering
    \includegraphics[width=0.9\textwidth]{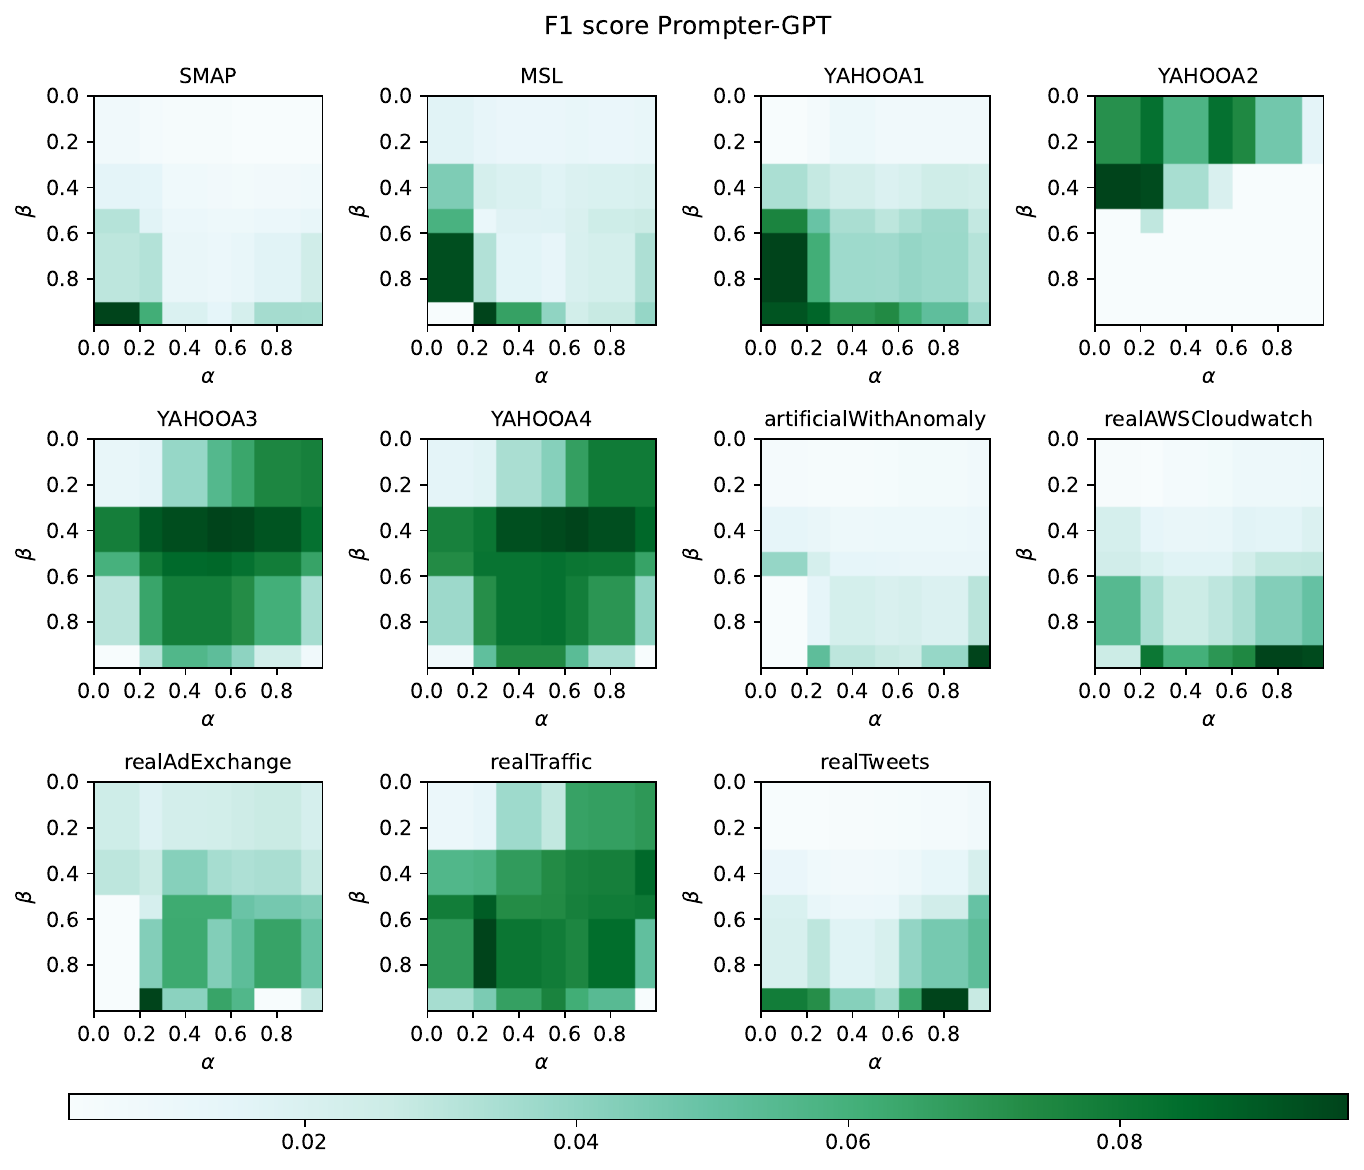}
    \caption{\prompt \gpt{} F1 score versus $\alpha$ and $\beta$ for each dataset.}
    \label{fig:gpt_prompter_dataset}
\end{figure*}

\begin{figure*}[ht]
    \centering
    \includegraphics[width=0.9\textwidth]{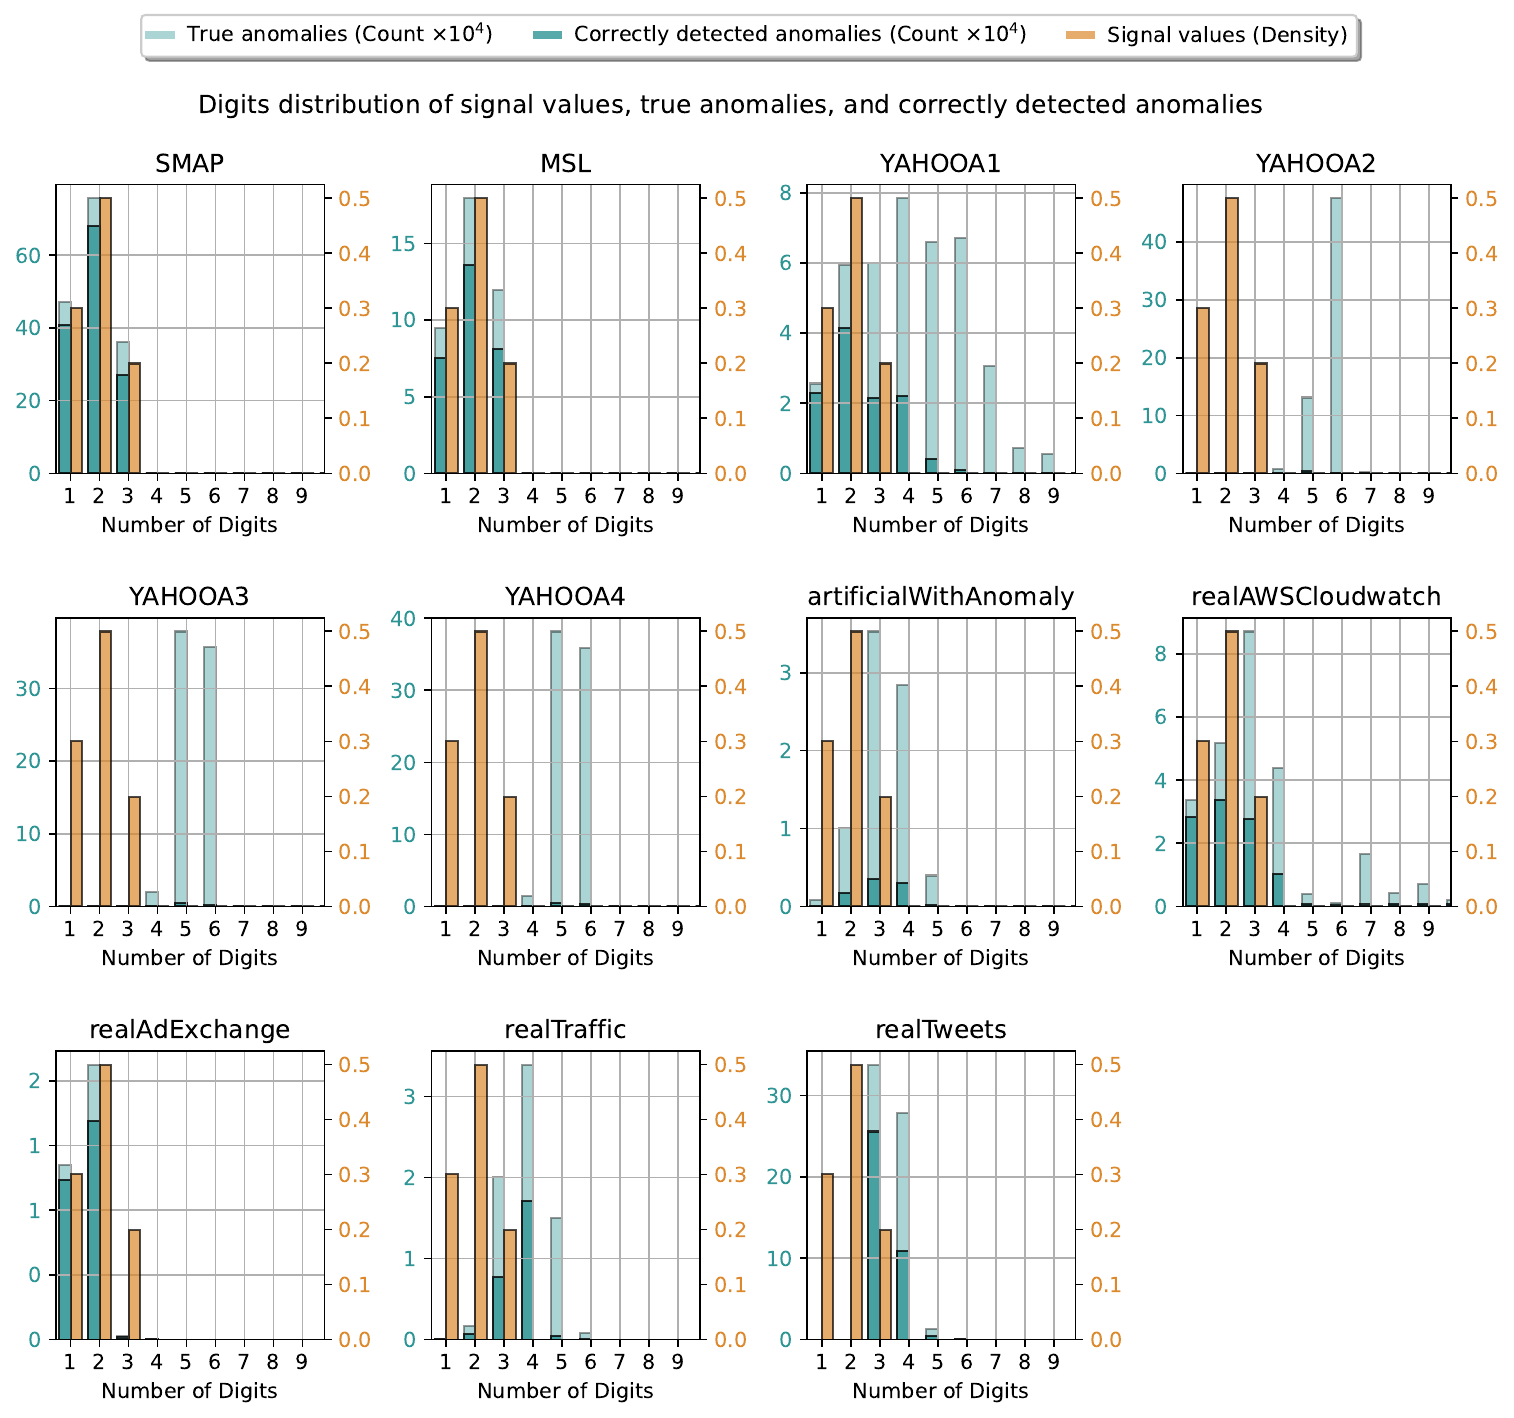}
    \caption{}
    \label{fig:mistral_digit_dist}
\end{figure*}

\begin{figure*}[ht]
    \centering
    \includegraphics[width=0.9\textwidth]{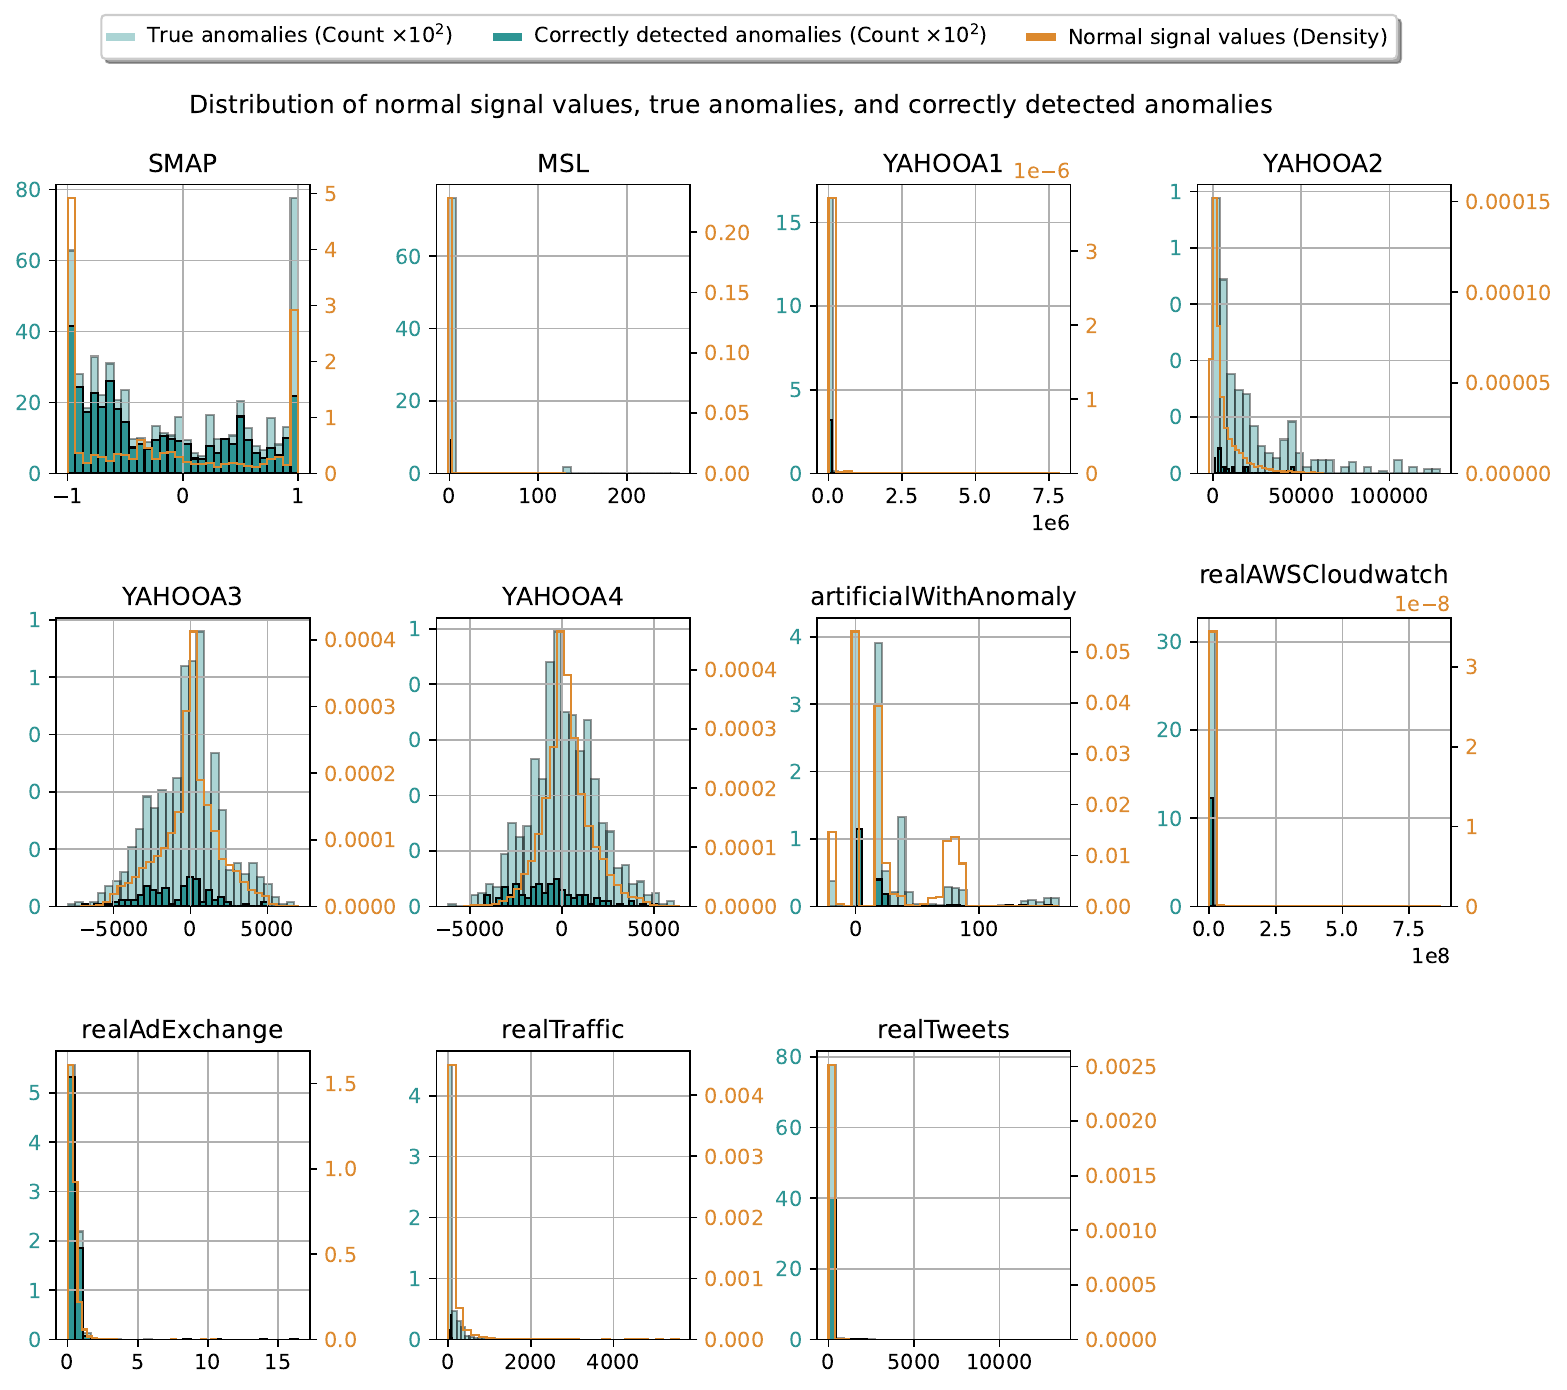}
    \caption{}
    \label{fig:mistral_dist}
\end{figure*}
